# Supplementary material for: Deep Fusion: Capturing Dependencies in Contrastive Learning via Transformer Projection Heads
Source: arXiv:2403.18681 source file (2024-10-07)
Supplement: Supplementary file 1 [file Appendix1-InfoNCE.tex]

\def \z{\mathbf{z}}
\def \Z{\mathbf{Z}}

In this section, we demonstrate its relationship with well-known InfoNCE \cite{wu2018unsupervised} in both self-supervised and supervised manner. Specifically,
for self-supervised learning, InfoNCE can be found in the form of:
\begin{align}
 \L_{\text{self}} = - \sum_{i \in I} \log \frac{\exp(\z_i^\top \z_{j(i)}/\tau)}{\sum_{i \neq a} \exp(\z_i^\top \z_b/\tau)} 
\end{align}
where $I$ denote the collection of samples from the current training batch; $\tau$ is a temperature constant; $\z_i$ is the feature extraced from i'th sample; $j(i)$ corresponding to the positive example of sample $i$, which is usually generated by augmentation of sample $i$. 

Since it's self-supervised learning, we know that there only exit 1 positive sample for each batch, which means that $|P(i)| = 1$, and $[\Y]_{ij}$ can only be either $0$ or $1$.
This means that the loss can be simplified to:
$$\L_{\text{TF}} :=  \D(\Y|| \sigma(\A^d/\tau)) = \sum_{i,j} [\Y]_{i,j} \log \frac{[\Y]_{i,j}}{[\sigma(\A^d/\tau)]_{i,j}} = \sum_{i \in I, j \in P(i)} -\log {[\sigma(\A^d/\tau)]_{i,j}}.$$ 

If we force the weight of Key and Query in the last layer to be the same $\W_Q^{d} = \W^d_{K} = \Tilde{\W}$, then we can have embeddings $\Z$ denote as:
$\Z := \X^\ell \Tilde{\W}$, and
$$[\sigma(\A^d/\tau)]_{i,j} = \frac{\exp(\z_i^\top \z_{j}/\tau)}{\sum_{i \neq a} \exp(\z_i^\top \z_b/\tau)} $$
which is exactly the same as $\L_{\text{self}}$.

For supervised learning manner, referring to \cite{khosla2020supervised}, the loss can be defined as
\begin{align}
    \mathcal{L}_{\text{sup}} =
\sum_{i \in I} \frac{-1}{|P(i)|} \sum_{p \in P(i)} \log \frac{\exp(\mathbf{z}_i^\top \mathbf{z}_p/\tau)}{\sum_{a \neq i} \exp(\mathbf{z}_i^\top \mathbf{z}_b/\tau)}
\label{sup_NCE}
\end{align}
where $P(i)$ denote the collection of samples from the same class as $i$'th sample. By pluging in \eqref{Y_def} to \eqref{L_TF}, it's trivial that $\mathcal{L}_{\text{sup}} = \L_{\text{TF}}$.
