# Supplementary material for: Deep Fusion: Capturing Dependencies in Contrastive Learning via Transformer Projection Heads
Source: arXiv:2403.18681 source file (2024-10-07)
Supplement: Supplementary file 2 [file Appendix4-Different_Loss.tex]

In this section, we undertake an empirical comparison among different loss functions. To conduct this comparison, we used CIFAR10 and trained a one-layer Transfusion model on top of a pretrained 18 Layer ResNet \cite{he2016deep}, employing each of the loss functions separately. Subsequently, we extracted the intermediate output from the ResNet as embeddings. These embeddings were then utilized to train a Support Vector Machine \cite{hearst1998support} on the training dataset, followed by performing classification on the embeddings from the test dataset. This procedure is a standard practice for evaluating the quality of the fixed embeddings, aligning with the recommendation provided by \cite{li2020prototypical}.

The Transfusion's training process follows a supervised contrastive learning approach, where the target affinity matrix is constructed based on the class labels of the samples. For this experiment, we did not introduce any augmentation techniques. To enhance training performance, the input images were resized from dimensions of $(32, 32, 3)$ to $(224, 224, 3)$.

Recall that one layer Transfusion model is essentially generating the cosine similarity between samples:
\begin{align}
    \A := (\Z\W_Q)(\Z\W_K)^\top
\end{align}
where $\Z \in \mathbb{R}^{n \times m}$ denotes the embeddings from the upstream ResNet18 model; $n$ denotes the number of samples; $m$ denotes the ambient dimension; $\W_Q, \W_K \in \mathbb{R}^{m \times m}$ denotes learn-able parameters. The loss functions we are interested are:

\begin{itemize}
    \item Supervised InfoNCE (KL-Divergence with Softmax) \eqref{sup_NCE}: $\L_{\text{KL-Softmax}}:= \D(\Y || \sigma(\A))$ 
    \item KL-Divergence with ReLU (KL-ReLU): $\L_{\text{KL-ReLU}}:= \D(\Y || \text{Normalize}(\A_+))$
    \item KL-Divergence with Squared Affinity (KL-Squared): $\L_{\text{KL-Squared}}:= \D(\Y || \text{Normalize}(\A^2))$
    \item Jensen-Shannon Divergence with Squared Affinity (JSD-Squared): $$\L_{\text{JSD-Squared}}:= \D(\Y || \text{Normalize}(\A^2)/2 + \Y/2) + \D(\text{Normalized}(\A^2) || \text{Normalize}(\A^2)/2 + \Y/2)$$
\end{itemize}
The outcomes for each of the loss functions are depicted in Figure \ref{Learning Rate}. 
From the results, it is evident that our custom loss function exhibits remarkable robustness across a broad spectrum of learning rates. It consistently maintains stable regions where classification accuracy remains consistently high. The next best performer is the KL-Squared, which shares similarities with the JSD-Squared. Notably, there are slight improvements when opting for JSD over KL.
In contrast, it becomes apparent that the KL-Softmax function displays a heightened sensitivity to variations in the learning rate. Across numerous trials, we encountered challenges such as overflows, even after normalizing the values prior to the Softmax operation.

\begin{figure}
    \centering
    \includegraphics[width = 0.65\textwidth]{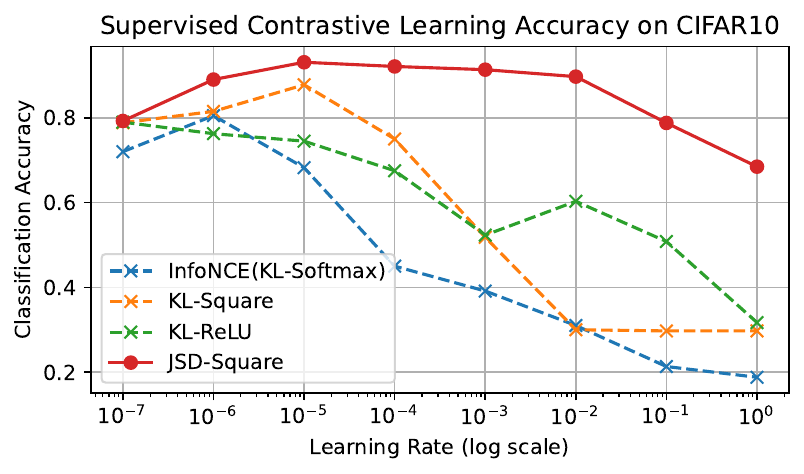}
    \caption{Precision in the encoding derived from a single-layer Transfusion model on top of ResNet18 \cite{he2016deep} with supervised contrastive learning.  This experiment was conducted on the CIFAR10 dataset, with ResNet18 pretrained on ImageNet1K as the underlying model.}
    \label{Learning Rate}
\end{figure}
