# Supplementary material for: Deep Fusion: Capturing Dependencies in Contrastive Learning via Transformer Projection Heads
Source: arXiv:2403.18681 source file (2024-10-07)
Supplement: Supplementary file 3 [file Appendix5-Code.tex]

\subsection{Model}

\begin{lstlisting}[style=mystyle]
class Transfusion(nn.Module):
    def __init__(self, num_layers, backbone):
        super(Transfusion, self).__init__()
        self.num_layers = num_layers

        # Backbone
        self.backbone = backbone
        self.num_ftrs  = self.backbone.fc.in_features
        self.backbone.fc = nn.Sequential([nn.Flatten(), nn.LayerNorm(self.num_ftrs)])

        # TransFusion
        self.attention_blocks = nn.Sequential(
            [TransFusionBlock(self.num_ftrs, self.num_ftrs) 
                for _ in range(num_layers)])


    def forward(self, x):
        x = self.backbone(x)
        if self.num_layers == 0:
            fused_embedding = embedding
        else:
            fused_embedding = self.attention_blocks(embedding)

        return fused_embedding



class TransFusionBlock(nn.Module):
    def __init__(self, input_size, output_size, activation):
        super(TransFusionBlock, self).__init__()
        self.input_size = input_size
        self.output_size = output_size

        # Learnable Weights
        self.query = nn.Linear(input_size, output_size)
        self.key = nn.Linear(input_size, output_size)
        self.value = nn.Linear(input_size, output_size)

        self.activation = nn.ReLU()

    def forward(self, x):
        q =  F.normalize(self.query(x))
        k =  F.normalize(self.key(x))
        v =  self.value(x)

        # Calculate Cosine Similarity
        attn_weights = torch.matmul(q, k.transpose(-2, -1))
        attn_weights = self.activation(attn_weights)

        # Normalize Weights
        attn_weights = attn_weights - torch.diag(torch.diagonal(attn_weights))
        attn_weights = (attn_weights + 1e-10) 
                    / torch.sum(attn_weights+1e-10, dim=1, keepdim=True)

        # Apply the attention weights to the value vectors
        output = torch.matmul(attn_weights, v) + x

        return output

\end{lstlisting}

\subsection{Loss Function}
\begin{lstlisting}[style=mystyle]

class Loss(nn.Module):
    def __init__(self):
        super(Loss, self).__init__()

    def forward(self, embeddings, target_affinity):
        # Normalize the input tensor
        normalized_zs = F.normalize(embeddings)

        # Compute the affinity matrix
        affinity = torch.matmul(normalized_zs, normalized_zs.transpose(-2, -1))
        affinity = affinity**2

        # Normalize Weights
        affinity = affinity - torch.diag(torch.diagonal(affinity))
        affinity = (affinity + 1e-10) 
                    / torch.sum(affinity+1e-10, dim=1, keepdim=True)
                    
        # Compute the JSD loss
        loss = F.kl_div((affinity+target_affinity).log(), 
                        target_affinity, 
                        reduction='batchmean')
        loss += F.kl_div((affinity+target_affinity).log(), 
                        affinity, 
                        reduction='batchmean')

        
        return loss

    
\end{lstlisting}
